# Supplementary material for: Neural Stochastic PDEs: Resolution-Invariant Learning of Continuous Spatiotemporal Dynamics
Source: arXiv:2110.10249 source file (2022-09-24)
Supplement: Supplementary file 1 [file split_appendix.tex]

\documentclass[letterpaper]{article}

\usepackage{pdfpages}

\usepackage{bashful}

\begin{document}

\bash
latexmk -pdf nature >& /dev/null
\END

%main
% \includepdf[pages=1-11]{nature}

%appendix
\includepdf[pages=12-]{nature}

\end{document}
